# Supplementary material for: Sample-Efficient Linear Representation Learning from Non-IID Non-Isotropic Data
Source: arXiv:2308.04428 source file (2024-10-12)
Supplement: Supplementary file 1 [file counterexamples.tex]

\section{Necessity of De-Biasing and Feature-Whitening}

We demonstrate in this section the issues with following the vanilla representation gradient, and thus the necessity of the proposed de-biasing and feature-whitening steps. The unifying theme is that missing either the de-biasing or feature-whitening steps on the local task-specific gradient update incurs a non-vanishing bias, thus bottlenecking the improvement of the representation at a level that cannot be improved no matter how many (independent) source tasks $H$ are used. To emphasize these fundamental issues, we make the following \textit{simplifying} features to the setting:
\begin{itemize}
    \item We assume the data distribution for each task is \textit{identical}: $\prob_{x,y}^{(h)} \equiv \prob_{x,y}$ for all $h \in [H]$.

    \item We assume no label noise is present $\whit \equiv 0$.

    \item We consider the \textit{infinite data} limit for each task, that is $n,T \to \infty$, removing any contribution from finite-data fluctuations.

\end{itemize}

We first assess the importance of the de-biasing step between

% Interaction of least-squares weights and representation update
