# Supplementary material for: Sample-Efficient Linear Representation Learning from Non-IID Non-Isotropic Data
Source: arXiv:2308.04428 source file (2024-10-12)
Supplement: Supplementary file 2 [file extended_discussion.tex]

\section{Extended Discussion}\label{sec: extended discussion}

\red{Necessity of $HNT$ rates for optimal online learning}

\red{Connections to stochastic bi-level optimization}

\red{Limitations of initialization and unbiasedness}

\red{Limitations: convergence rate. Proposed practical solution: adaptive law based on gradient norm / momentum}

\red{(might be too subtle) Realizability for linear vs non-linear features. NNs can get 0 empirical loss on random data; should imply that NNs can get 0 empirical loss on random non-linear features?}
